# Supplementary material for: Action-based image editing guided by human instructions
Source: arXiv:2412.04558 source file (2025-02-04)
Supplement: Supplementary file 1 [file X_suppl.tex]

\clearpage
\setcounter{page}{1}
\maketitlesupplementary

\section{The selection of $\lambda_1$ and $\lambda_2$}\label{sec:editaction_hyperparamets}
section \cref{implementation}
To select the hyperparameters $\lambda_1$ and $\lambda_2$, we use FID score to rank models trained on 1000 training steps with $\lambda_1, \lambda_2 \in \{10^{-4}, 30^{-4}, 50^{-4}, 10^{-3}, 30^{-3}, 50^{-3}, 10^{-2}, 30^{-2}, 50^{-2}\}$. As observed in Figure~\ref{fig:parameters}, $\lambda_1$ and $\lambda_2$ are set to $50^{-4}$ and $30^{-2}$. \textcolor{blue}{To select the best $\lambda_1$ value, we train our model using only the $\mathbf{L}_{action}$ loss. Similarly, the best $\lambda_2$ value is selected by including only the $\mathbf{L}_{reg}$ loss during the training.}

\begin{figure}[t]
    \centering
    \includegraphics[width=8cm]{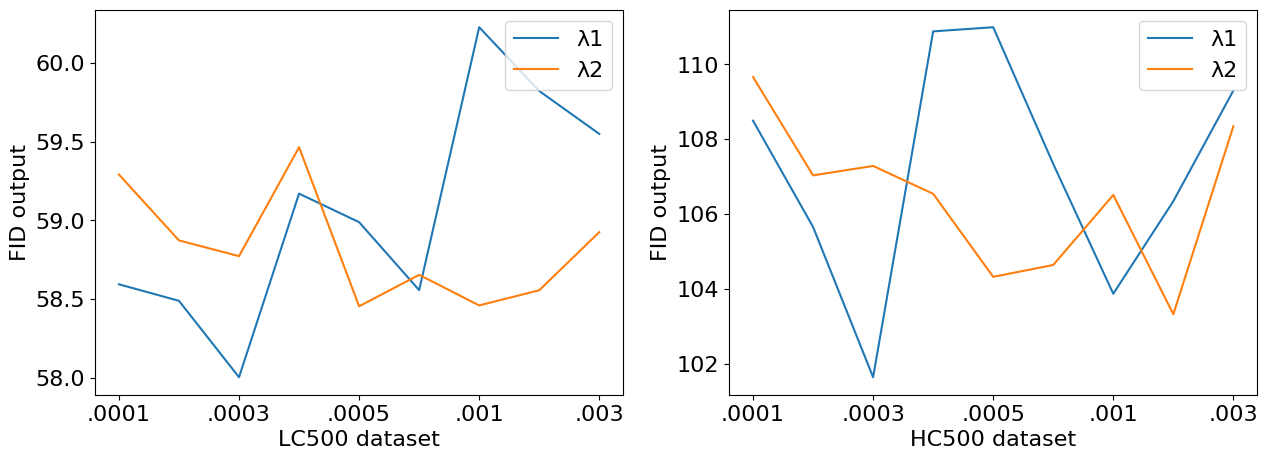}
    \caption{The selection of $\lambda_1$ and $\lambda_2$ hyperparameters based on the FID score. Considering the results reported for LC and HC datasets, the optimal values for $\lambda_1$ and $\lambda_2$ are $50^{-4}$ and $30^{-2}$, respectively.
    }
    \label{fig:parameters}
\end{figure}

\section{Rationale}
\label{sec:rationale}
Having the supplementary compiled together with the main paper means that:
\begin{itemize}
\item The supplementary can back-reference sections of the main paper, for example, we can refer to \cref{sec:intro};
\item The main paper can forward reference sub-sections within the supplementary explicitly (e.g. referring to a particular experiment); 
\item When submitted to arXiv, the supplementary will already included at the end of the paper.
\end{itemize}
To split the supplementary pages from the main paper, you can use \href{https://support.apple.com/en-ca/guide/preview/prvw11793/mac#:~:text=Delete%20a%20page%20from%20a,or%20choose%20Edit%20%3E%20Delete).}{Preview (on macOS)}, \href{https://www.adobe.com/acrobat/how-to/delete-pages-from-pdf.html#:~:text=Choose%20%E2%80%9CTools%E2%80%9D%20%3E%20%E2%80%9COrganize,or%20pages%20from%20the%20file.}{Adobe Acrobat} (on all OSs), as well as \href{https://superuser.com/questions/517986/is-it-possible-to-delete-some-pages-of-a-pdf-document}{command line tools}.
